# Supplementary material for: AdvDreamer Unveils: Are Vision-Language Models Truly Ready for Real-World 3D Variations?
Source: arXiv:2412.03002 source file (2025-03-09)
Supplement: Supplementary file 1 [file supp.tex]

% % \clearpage
% \setcounter{page}{1}
% \maketitlesupplementary
\section*{Overview}
This supplementary material provides some essential details that complement our main paper. Sec.~\ref{sec:a} presents the mathematical derivation of the AdvDreamer distribution update formulation, which builds upon the canonical form of CMA-ES~\cite{hansen2016cma,golovin2017google}. Sec.~\ref{sec:b} provides detailed experimental settings and results. Specifically, Sec.~\ref{sec:b1} details the implementation of AdvDreamer and the configuration of critical hyperparameters. Sec.~\ref{sec:b2} presents a comprehensive ablation study quantifying the impact of NRM feedback on Adv-3DT's naturalness. Sec.~\ref{sec:b3} offers additional results and analysis of physical experiments. Sec.~\ref{sec:b4} provides the computational cost of AdvDreamer. Sec.~\ref{sec:b5} provides a comparison of Adv-3DT samples from AdvDreamer with those from previous studies. Sec.~\ref{sec:c} provides all prompt templates provided to GPT-4 for automatic annotation of naturalness datasets and GPT-Score / GPT-Acc metrics. Sec.~\ref{sec:d} showcases additional visualization of Adv-3DT examples and its performance across various tasks. Finally, Sec.~\ref{sec:e} provides an in-depth description of MM3DTBench and presents detailed quantitative benchmarking results. Sec.~\ref{sec:f} reports the ImageNet categories utilized in experiments and examples of clean images.

\section*{Open Source Declaration}
We will release the source code of AdvDreamer, along with the MM3DTBench dataset and the evaluation scripts. We will also release our naturalness reward model's weights and training dataset. We believe these open-source contributions will facilitate future research in VLMs' 3D variation robustness evaluation.

\begin{table*}[t]
\caption{Category-wise accuracy (\%) of physical Adv-3DT samples under different tasks.}
\vspace{-0.1cm}
\setlength\tabcolsep{2.0pt}

\centering
\scalebox{0.85}{
\begin{tabular}{ccccccccccccc}
\hline
Task              & airliner & ambulance & fire truck & forklift & water jug & laptop & police van & shoe  & street sign & tank & traffic light & trash bin \\ \hline
Zero-shot Cls.    & 49.4     & 68.4      & 1.0        & 85.0     & 0.0       & 99.5   & 25.3       & 100.0 & 48.2        & 90.9 & 47.2          & 0.4       \\ \hline
VQA-Choice        & 3.1      & 35.9      & 67.2       & 9.4      & 0.0       & 99.5   & 34.7       & 100.0 & 57.2        & 5.3  & 0.6           & 26.3      \\ \hline
VQA-Ture or False & 0.3      & 14.1      & 0.5        & 37.2     & 99.5      & 99.5   & 2.6        & 100.0 & 96.4        & 85.2 & 0.3           & 58.8      \\ \hline
\end{tabular}}
\label{phy details}
\end{table*}

\section{Details of Optimization Algorithm} \label{sec:a}

\subsection{Derivation of Eq.(\textcolor{cvprblue}{10}) \& (\textcolor{cvprblue}{11})}\label{sec:a1}

AdvDreamer optimizes adversarial 3D transformation distributions through Covariance Matrix Adaptation Evolution Strategy (CMA-ES). Among various evolutionary optimization algorithms, CMA-ES stands out as one of the most prominent and effective approaches, demonstrating superior performance particularly on medium-scale optimization problems (typically involving 3-300 variables)~\cite{golovin2017google}. Its gradient-free nature eliminates the dependency on gradient information, making it an ideal choice for optimizing the adversarial 3D transformation distributions in AdvDreamer.

Following the canonical formulation of CMA-ES, AdvDreamer generates a population of 3D transformations in each optimization iteration $t$ by sampling from the current adversarial distribution with a specified step size $\boldsymbol{\sigma}^t$, formally expressed as:
\begin{equation}
    \boldsymbol{z}_i = \boldsymbol{\mu}^t+\boldsymbol{\sigma}^t\cdot \boldsymbol{\gamma}_i~~\text{where}~\boldsymbol{\gamma}_i\sim \mathcal{N}(0,\boldsymbol{\Sigma}^t),
\end{equation}
where each $\boldsymbol{\gamma}_i$ represents a search direction in the transformation space. The sampling process for $\boldsymbol{\gamma}_i$ can be performed through either Eigendecomposition of the current adversarial distribution's covariance matrix $\boldsymbol{\Sigma}^t= BD^2B^T$, or Cholesky decomposition, followed by transformation of samples drawn from a standard normal distribution:
\begin{equation}
    \boldsymbol{\gamma}_i=BD\boldsymbol{\delta}_i,~~\text{where} ~{\delta}_i\sim \mathcal{N}(0,\textbf{I}).
\end{equation}
The sampled population $\{\boldsymbol{z}_i\}_{i=1}^K$ undergoes reparameterization to obtain a constrained set of 3D transformation parameters $\{\boldsymbol{\Theta}_i\}_{i=1}^K$, as formulated in Eq.(\textcolor{cvprblue}{8}). By applying $\{\boldsymbol{\Theta}_i\}_{i=1}^K$ to the original images under generative process, we generate a batch of Adv-3DT samples $\{X'_i\}_{i=1}^K$ and compute their $\mathcal{L}_\text{Nat}$ and $\mathcal{L}_\text{IPS}$ losses. The samples are then ranked according to their $\mathcal{L}_\text{IPS}$ values, which quantify the adversarial effectiveness against the target model:
\begin{equation}
\mathcal{L}_\text{IPS}\left(X'_{1: K}\right) \leq \mathcal{L}_\text{IPS}\left(X'_{2: K}\right) \leq \cdots \leq \mathcal{L}_\text{IPS}\left(X'_{k: K}\right).
\end{equation}
We employ truncation selection to identify the samples contributing to distribution parameter updates. Specifically, we select the $k$ most adversarial samples based on $\mathcal{L}_\text{IPS}$ scores, then retain the top $k/2$ samples with the highest $\mathcal{L}_\text{Nat}$ values. This two-stage selection mechanism effectively serves as a naturalness regularization for the optimization process. For the sake of simplicity, we denote this selected subset of population as $\{\textbf{z}_{(i:k)}\}_{i=1}^k$ and utilize it to update both the distribution parameters $\boldsymbol{\mu}^{t+1}, \boldsymbol{\Sigma}^{t+1}$ and step size $\boldsymbol{\sigma}^{t+1}$. The updated mean of the distribution is computed as the weighted maximum likelihood estimate of the selected population, which can be expressed as:  
\begin{equation} \label{update mu}
\boldsymbol{\mu}^{t+1} = \sum_{i=1}^{k}w_i\cdot \mathbf{z}_{(i:k)}^{t+1},~~\text{where}~\sum_{i=1}^{k}w_i = 1.
\end{equation}
This formulation indicates that the updated mean shifts along the average search direction. In our implementation, we assign uniform weights to all selected population, where $w_i= 1/k$.  The covariance matrix $\boldsymbol{\Sigma}$ update comprises both rank-1 and rank-$\mu$ terms. The rank-1 term incorporates historical search information through an evolution path, which is constructed as:
\begin{equation} 
p_{t+1}=(1-c) p_{t}+\sqrt{c(2-c)} \sqrt{\mu_{w}} \frac{\boldsymbol{\mu}^{t+1}-\boldsymbol{\mu}^{t}}{\boldsymbol{\sigma}_{t}},
\end{equation}
where the factor $\mu_{w}=\frac{1}{\sum_{i=1}^{k} w_{i}^{2}}$, $c$ represents the adaptation rate/learning rate, is designed based on $c^{-1} \propto n$. Notably, $c$ is inversely proportional to the degrees of freedom (number of parameters) of the adjustable variables. The evolution path characterizes the movement of the distribution mean by maintaining an exponentially weighted average of the update directions $\frac{\boldsymbol{\mu}^{t+1}-\boldsymbol{\mu}^{t}}{\boldsymbol{\sigma}_{t}}$ across iterations. This path effectively encodes one of the most promising search directions in the current optimization landscape.  The covariance matrix update is based on:
\begin{equation}
\operatorname{argmax} p\left(p_{t+1} \mid \boldsymbol{\mu}, \boldsymbol{\Sigma}\right), \operatorname{argmax} \prod_{i=1}^{k} p\left(\left.\frac{\textbf{z}_{(i:k)}-\boldsymbol{\mu}^{t}}{\boldsymbol{\sigma}^{t}} \right\rvert\, \boldsymbol{\mu}, \boldsymbol{\Sigma}\right).
\end{equation}
Building upon this principle, the update rule can be formulated as: 
\begin{equation}
\begin{gathered} \label{sigma}
\boldsymbol{\Sigma}^{t+1} = (1-\eta_1-\eta_{\mu})\cdot\boldsymbol{\Sigma}^t+\eta_1\cdot p^{t+1}_{\Sigma}(p^{t+1}_{\Sigma})^T+ \\
\eta_{\mu}\cdot\sum_{i=1}^{h}w_i\cdot(\frac{\mathbf{z}_{(i:k)}^{t+1}-\boldsymbol{\mu}^{t}}{\boldsymbol{\sigma}^t})(\frac{\mathbf{z}_{(i:k)}^{t+1}-\boldsymbol{\mu}^{t}}{\boldsymbol{\sigma}^t})^T.
\end{gathered}
\end{equation}
This update mechanism effectively increases the sampling probability along successful search directions by expanding the variance in these directions.  The rank-1 term in Eq.~\eqref{sigma}, as previously mentioned, directly leverages the evolution path as a successful search direction. The second term (rank-$\mu$), represents the weighted maximum likelihood estimate of the selected population, which can be interpreted as natural gradient optimization of $\boldsymbol{\Sigma}$ in the information geometry framework. The learning rates $\eta_1, \eta_{\mu}$ for both terms follow the same design principle as $c_{1} \approx \frac{2}{n^{2}}, c_{\mu} \approx \frac{\mu_{w}}{n^{2}}$, where they are inversely proportional to the degrees of freedom (number of parameters) of the adjustable variables.

For step size $\boldsymbol{\sigma}$ adaptation, we adopt the Cumulative Step-size Adaptation (CSA) mechanism, which is widely recognized as the most successful and prevalent approach in the CMA-ES framework~\cite{chotard2012cumulative, chotard2015markov}. The above derivations provide a comprehensive elaboration of the algorithmic details presented in Sec.~\textcolor{cvprblue}{3.5} of the main paper. 

\subsection{Pseudocode of AdvDreamer Framework}\label{sec:a2}
We provide the pseudocode for AdvDreamer in Algorithm~\ref{algorithm}

\begin{algorithm}[t] \small
\setstretch{0.3}
\caption{\small Optimization Algorithm of AdvDreamer}\label{algorithm}
\KwData{Natural images or text descriptions $I\in\{X, T\}$.}
\KwResult{Optimal distribution parameters $\boldsymbol{\mu}^*,\boldsymbol{\Sigma}^*$.}
\tcc{\scriptsize Foreground-Background Pairs Preparation}
$\{X_f,X_b \}\leftarrow \mathcal{F}(I)$\; 
\tcc{\scriptsize Initialization of distribution parameters}
$\boldsymbol{\mu}^0 \leftarrow \mathbf{0}$, $\boldsymbol{\Sigma}^0 \leftarrow \mathbf{I}$\;
\While{$t<t_{\max}$}{
\tcc{\scriptsize Generate a batch of adversarial samples}
    \For{$i=1 \to K$}{
$\mathbf{z}^{t+1}_i \sim \mathcal{N}(\boldsymbol{\mu}^t,\boldsymbol{\Sigma}^t)$\;
$\boldsymbol{\Theta}^{t+1}_i \leftarrow \mathbf{A}\cdot\tanh(\mathbf{z^{t+1}_i})+\mathbf{B}$\;
$(X')^{t+1}_i \leftarrow \mathcal{C}_{\textbf{w}_1}(\mathcal{R}_{\textbf{w}_0} (X_f, \boldsymbol{\Theta}^{t+1}_i),X_b)$\;
\tcc{\scriptsize Calculate loss/fitness value} 
$\mathcal{L}_i^{t+1} = \mathcal{L}_{\text{IPS}}((X')^{t+1}_i,\mathcal{Y})+\lambda\cdot\mathcal{L}_{\text{Nat}}((X')^{t+1}_i)$\;
}
Sorting $\mathcal{L}_i^{t+1}$ in ascending order\;
Obtain $\boldsymbol{\mu}^{t+1},\boldsymbol{\Sigma}^{t+1}$ by Eq.\eqref{update mu} and \eqref{sigma}\;
}
% Optimal Adv. transformation $\boldsymbol{\Theta}^* \leftarrow \mathbf{A}\cdot\tanh(\mathbf{\boldsymbol{\mu}^t_{\max}})+\mathbf{B}$\;
% Optimal Adv. transformation distribution  $p^*(\boldsymbol{\Theta}) \leftarrow p()$

% \mathbf{A}\cdot\tanh(\mathbf{\boldsymbol{\mu}^t_{\max}})+\mathbf{B}$
$\boldsymbol{\mu}^* \leftarrow \boldsymbol{\mu}^{t_{\max}},\boldsymbol{\Sigma}^* \leftarrow \boldsymbol{\Sigma}^{t_{\max}}$.
\end{algorithm}

\begin{table}[t]
\caption{The computational cost of AdvDreamer across different stages and total optimization process.}
\vspace{-0.1cm}
\setlength\tabcolsep{3.0pt}

\centering
\scalebox{0.8}{
\begin{tabular}{c|c|c|c|c|c}
\hline
          & Step.0 & Step.1@iter & Step.2@iter & Step.3@iter & Toatal   \\ \hline
Time Cost & $\le$1s    & $\sim$0.6s*k   & $\sim$6s*k     & $\le$1s         & $\sim$16.5min \\ \hline
\end{tabular}}
\label{time}
\end{table}

\begin{table}[t]
\caption{Computational Cost and Accuracy of Naturalness Assessment Across Human, GPT, and NRM Evaluations.}
\setlength\tabcolsep{3.0pt}

\centering
\scalebox{0.8}{
\begin{tabular}{c|c|c|c}
\hline
          & Human    & GPT-4o & NRM    \\ \hline
Time cost & $\sim$43min & $\sim$4min  & $\sim$5s    \\ \hline
Acc.      & -        & 64.94\% & 67.82\% \\ \hline
\end{tabular}}
\label{NRM1}
\end{table}

% \begin{table}[t]
% \caption{Attack Success Rate (ASR), visual realism score ($Score_R$) and physical plausibility score ($Score_P$) of Adv-3DT Samples with and without NRM.}
% \setlength\tabcolsep{5.0pt}
% \renewcommand\arraystretch{1.0}
% \centering
% \scalebox{0.8}{
% \begin{tabular}{c|c|c|c}
% \hline
%   Methods                  & ASR  & $Score_R$ & $Score_P$ \\ \hline
% AdvDreamer w/o. NRM & \textbf{51.4}\% & 1.60     & 1.39    \\ \hline
% AdvDreamer w/. NRM  & 47.2\% & \textbf{2.52}    & \textbf{2.57}    \\ \hline
% \end{tabular}}
% \label{NRM2}
% \end{table}

\begin{table*}[t]
\caption{The selected 30 categories in ImageNet dataset.}
\vspace{-0.1cm}
\setlength\tabcolsep{6.0pt}

\centering
\scalebox{0.8}{
\begin{tabular}{c|c|c|c|c|c|c|c|c|c|c|c}
\hline
0 & backpack      & 5 & carton    & 10 & rocking chair   & 15 & beaker      & 20 & coffee mug & 25 & monitor  \\ \hline
1 & barber chair  & 6 & chest     & 11 & lamp            & 16 & convertible & 21 & ballpoint  & 26 & dustcart \\ \hline
2 & minivan       & 7 & moped     & 12 & cocktail shaker & 17 & park bench  & 22 & waggon     & 27 & cleaver  \\ \hline
3 & folding chair & 8 & microwave & 13 & ambulance       & 18 & jug         & 23 & moving van & 28 & mailbox  \\ \hline
4 & hatchet       & 9 & coffeepot & 14 & fire truck      & 19 & crate       & 24 & chiffonier & 29 & doormat  \\ \hline
\end{tabular}}
\label{imagenet class}
\end{table*}
\section{Selected ImageNet Categories}\label{sec:f}
We conduct experiments of zero-shot classification task (Tab.~\textcolor{cvprblue}{1 }) on 30 ImageNet Categories, generating Adv-3DT samples from both ImageNet test set images and synthetic images created using Stable-Diffusionv2. The selected categories are enumerated in Tab.~\ref{imagenet class}.

\begin{table}[t]
\caption{VQA accuracy(\%) of representative VLMs under MM3DTBench.}
\vspace{-0.1cm}
\setlength\tabcolsep{4.0pt}

\centering
\scalebox{0.85}{
\begin{tabular}{l|ccc|c}
\hline
VLMs            & Choice & Free Answer & Avg.  & Rank \\ \hline
GPT-4o~\cite{gpt-4o}          & 69.30  & 47.44       & 58.37 & 1    \\
GPT-4o-mini~\cite{gpt-4o}     & 58.60  & 46.51       & 52.56 & 2    \\
CogVLM~\cite{wang2023cogvlm}          & 60.00  & 40.00       & 50.00 & 3    \\
InternVL~\cite{chen2024internvl}        & 46.05  & 49.77       & 47.91 & 4    \\
Qwen-VL~\cite{bai2023qwen}         & 58.60  & 36.74       & 47.67 & 5    \\
LLaVa-1.6~\cite{liu2024llavanext}       & 49.77  & 34.42       & 42.10 & 6    \\
ShareGPT-4V~\cite{chen2023sharegpt4v} & 50.23  & 33.02       & 41.63 & 7    \\
MiniGPT-4~\cite{zhu2023minigpt}       & 48.84  & 30.70       & 39.77 & 8    \\
Mplug-Owl2~\cite{ye2024mplug}      & 40.47  & 32.56       & 36.52 & 9    \\
InternLM-2~\cite{team2023internlm}      & 38.60  & 27.90       & 33.25 & 10   \\
LLaVa-1.5~\cite{liu2024visual}       & 41.40  & 24.60       & 33.00 & 11   \\
Claude-3~\cite{claude-3}        & 35.81  & 24.19       & 30.00 & 12   \\
LRV-Instruction~\cite{liu2023aligning} & 23.70  & 13.02       & 18.36 & 13   \\ \hline
\end{tabular}}
\label{bench}
\end{table}

\section{Additional Experimental Results}\label{sec:b}

\subsection{Implementation Details}\label{sec:b1}
\noindent\textbf{Optimization Algorithm.} we employ CMA-ES through the cmaes~\cite{nomura2024cmaes} library. The distribution mean $\boldsymbol{\mu}$ is initialized as $[90, 180, 90, 0, 0, 1.0]$, with optimization bounds constrained to $\boldsymbol{\Theta}_{\min}=[0, 160, 80, -100, -100, 0.5]$, $\boldsymbol{\Theta}_{\max}=[360, 200, 100, 100, 100, 1.5]$. We initialize covariance matrix $\boldsymbol{\mu}$ as a identity matrix, with a step size $\boldsymbol{\sigma}$ of 0.5, which decays exponentially during optimization with a decay rate of 0.9. Other hyperparameters follow the default configuration in official implementation.

\noindent\textbf{Training Details of NRM.}
To train the Natural Reward Model (NRM), we first establish a large-scale image naturalness assessment dataset, which comprises 100k images obtained by applying random 3D transformations to samples from ImageNet and generated images. Following the methodology detailed in Sec.~\textcolor{cvprblue}{3.4} of main paper, we leverage GPT-4o for automated naturalness scoring, complemented by human verification. Representative examples of the annotation process are illustrated in Fig.~\ref{fig:nat}. The dataset is split into training and validation sets with a 9:1 ratio.

We formulate NRM training as a multi-classification task, where the model predicts specific scores for realism and physical plausibility. The backbone of NRM adopts DINOv2 (ViT-L/14 distilled), where we apply average pooling over patch tokens to obtain 1024-dimensional feature representations. These features are then fed into two separate prediction heads for parallel classification. Each head consists of two fully connected layers with non-shared weights, configured as (1024, 512) and (512, 5), respectively. The network is optimized using cross-entropy loss as the training objective. The NRM is trained for 100 epochs, achieving a prediction accuracy of 75.03\% on the test set.

\subsection{Naturalness Evaluation Effect}\label{sec:b2}
\noindent\textbf{Alignment between NRM and Human Evaluation:} A critical aspect of NRM is its ability to approximate human judgment for replacing manual Adv-3DT image filtering during optimization. To validate this alignment, we conducted a human evaluation study on 175 test images with volunteer annotators. Tab.~\ref{NRM1} presents the agreement rates (difference within 1 point) between human scores and predictions from both NRM and GPT-4o. NRM achieves 67.82\% accuracy, outperforming GPT-4o's 64.94\%. This superior performance stems from additional manual refinement of NRM's training data to mitigate the inherent output instability of GPTs. Furthermore, Tab.~\ref{NRM1} demonstrates that NRM's inference time is negligible compared to both human and GPT-based evaluations, significantly enhancing optimization efficiency.

\begin{figure*}[t]
  \centering
  \includegraphics[height=14.9cm]{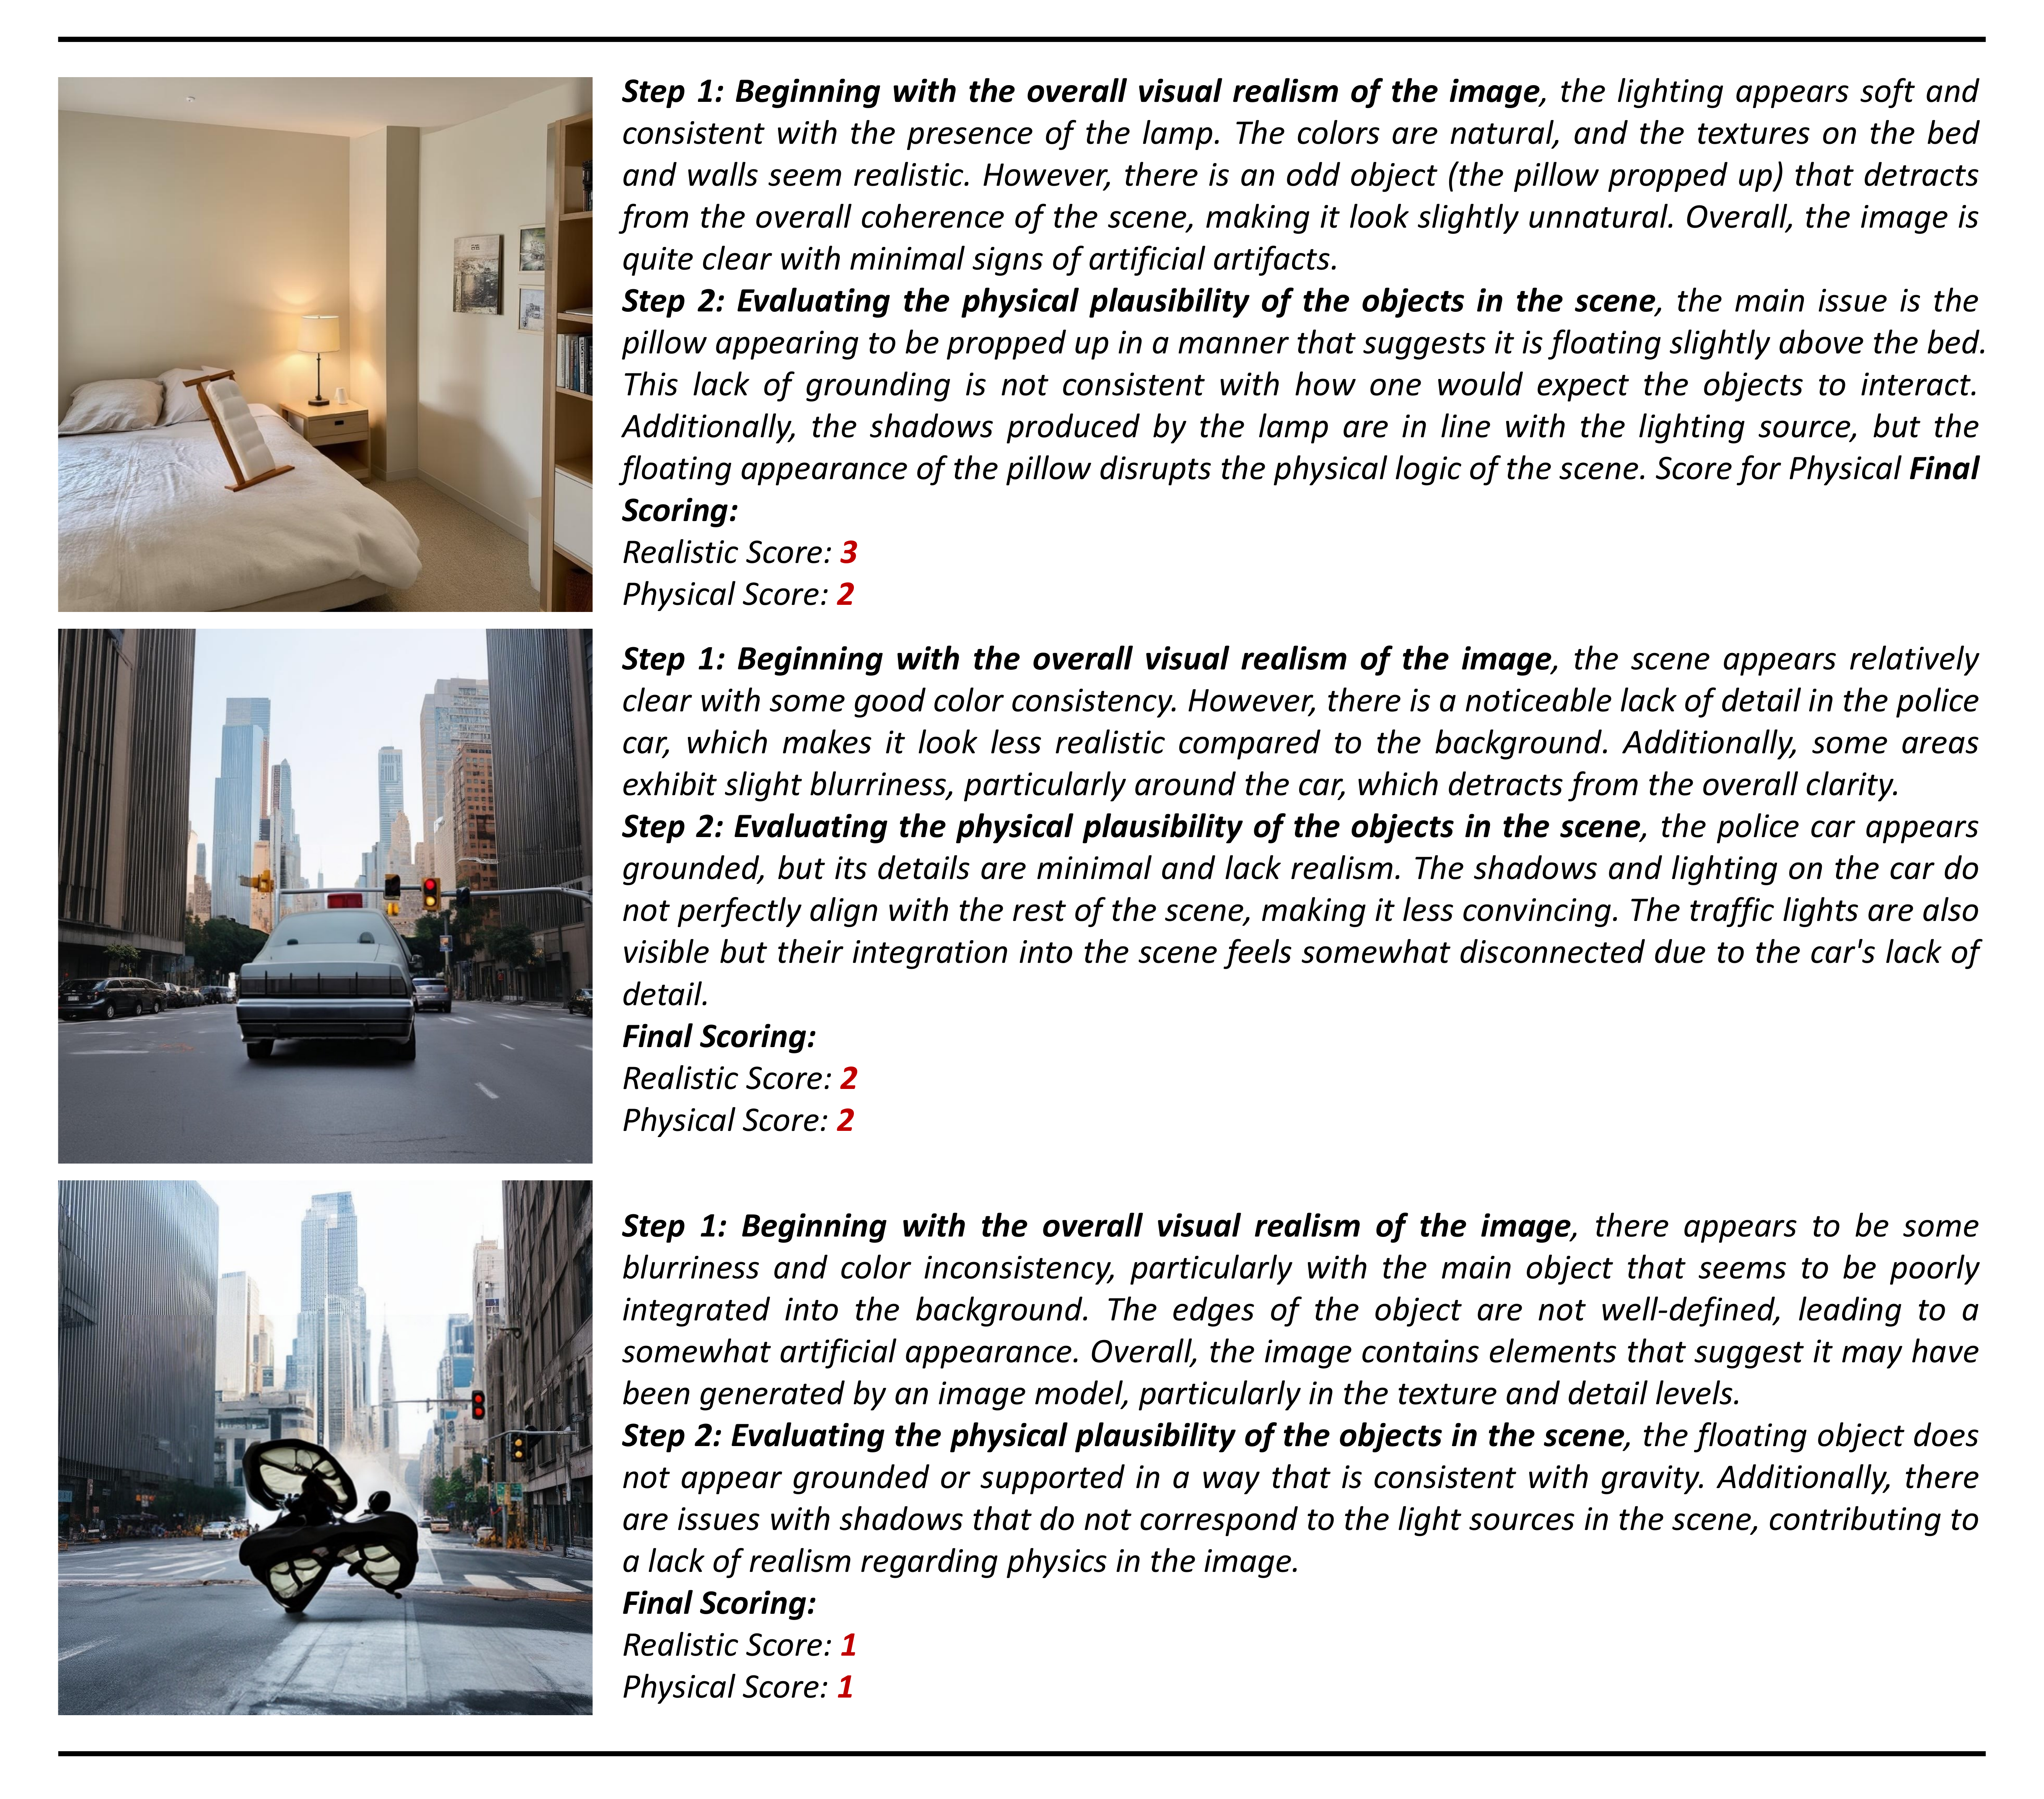}
  \caption{Examples of image naturalness annotation results using GPT-4o.}
  \label{fig:nat}
\end{figure*}

\subsection{Detailed Physical Experiment Results}\label{sec:b3}
Tab.~\ref{phy details} presents a detailed category-wise accuracy of our physical-world experiments (Tab.~\textcolor{cvprblue}{4} of main paper). Additionally, we visualize the zero-shot classification results using OpenCLIP ViT-B/16 on sampled frames (every 5 frames) from our physical reproduction vedio sequences, as shown in Fig.~\ref{fig:vis-2}. Green and red boxes indicate successful and failed classifications, respectively.

\begin{figure*}[t]
  \centering
  \includegraphics[height=13.9cm]{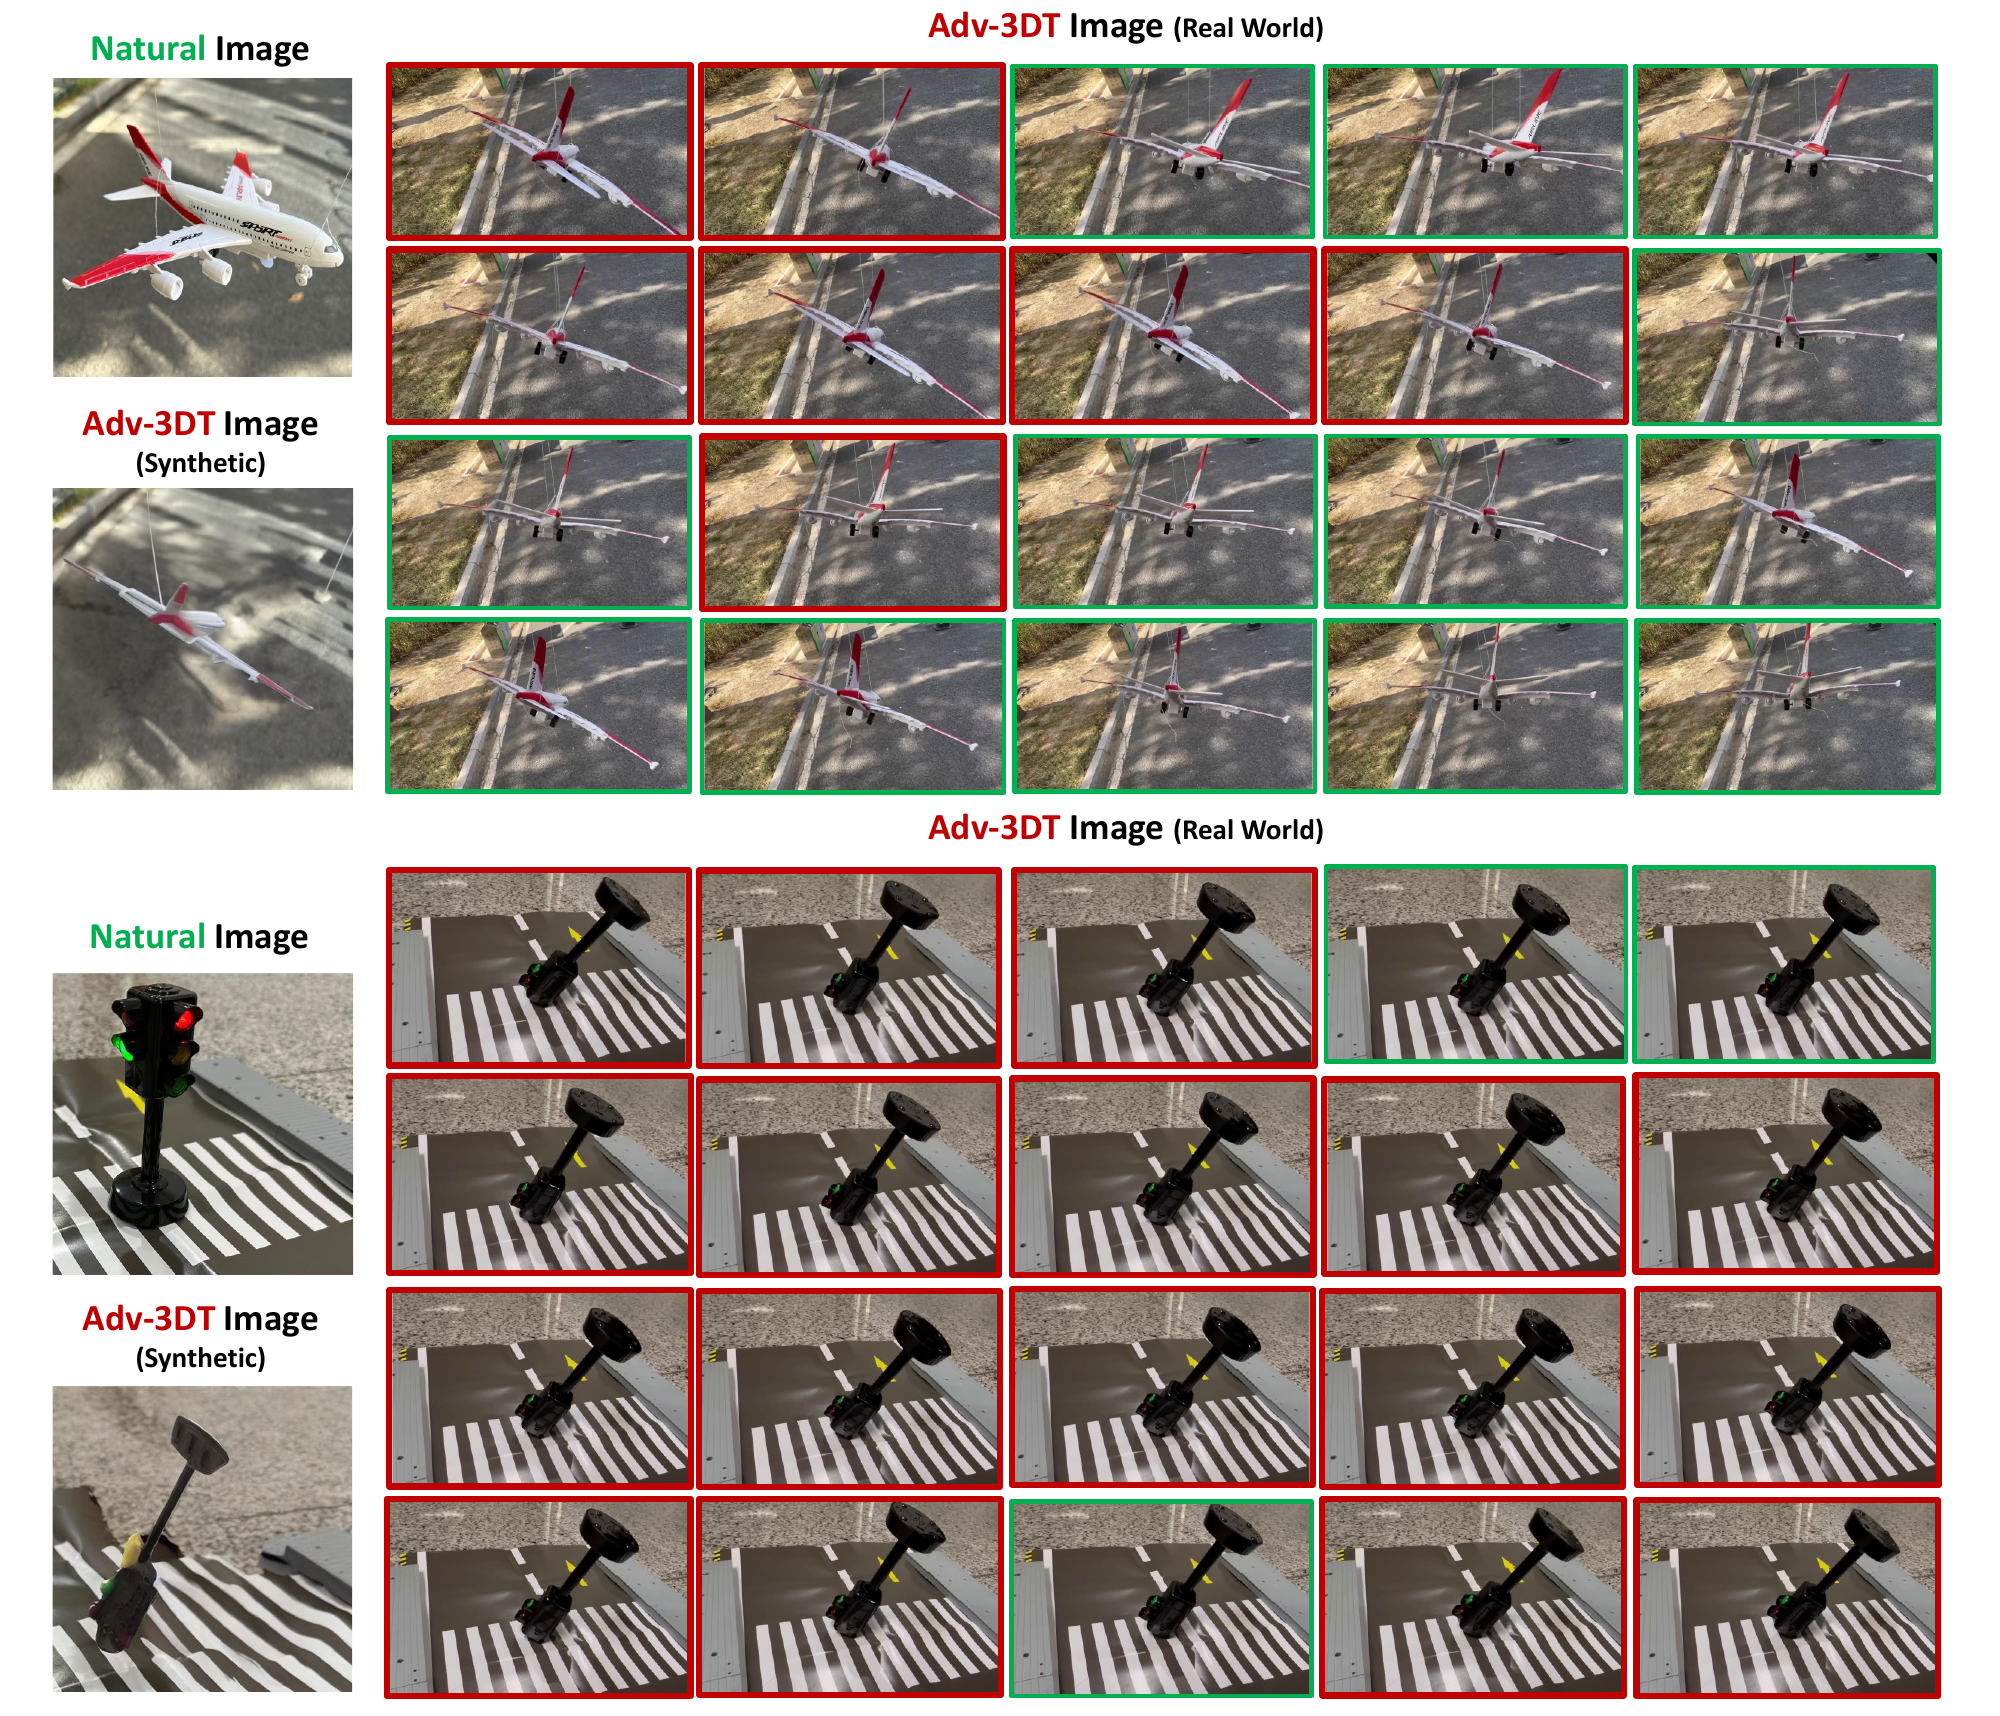}
  \caption{Physical reproduction results of Adv-3DT Samples: zero-shot classification performance on video frame sequences.}
  \label{fig:vis-2}
\end{figure*}

\subsection{Computational Cost}\label{sec:b4}

The computational overhead for different stages within a single iteration of AdvDreamer is detailed in Tab.~\ref{time}. For each clean sample, optimizing the adversarial distribution requires approximately 16.5 GPU minutes, with image reconstruction (step-2) being the primary bottleneck. Our experiments on the ImageNet test set (300 samples) consumed 96 GPU hours on an NVIDIA RTX 3090.

\subsection{Comparison with Prior Studies}\label{sec:b5}
We evaluate samples generated by different methods in overlapping ImageNet classes. The Tab.~\ref{sample compare} shows that AdvDreamer outperforms in both attack success rate (ASR) and naturalness ($Score_{R}$ and $Score_{P}$, defined in Eq.~(\textcolor{red}{6})).

\begin{table}[t]
\caption{comparison of Adv-3DT samples from AdvDreamer with those from previous studies.}
\vspace{-0.1cm}
\setlength\tabcolsep{2.5pt}

\centering
\scalebox{0.7}{
\begin{tabular}{l|c|cc|c|c}
    \hline
    \multirow{2}{*}{Method} & \multirow{2}{*}{Domain} & \multirow{2}{*}{\begin{tabular}[c]{@{}c@{}}ASR($\uparrow$)\\ (OpenCLIP)\end{tabular}} & \multirow{2}{*}{\begin{tabular}[c]{@{}c@{}}ASR($\uparrow$)\\ (BLIP-2)\end{tabular}} & \multirow{2}{*}{$Score_R$($\uparrow$)} & \multirow{2}{*}{$Score_P$($\uparrow$)} \\
                        &                         &                                                                                &                                                                              &                           &                           \\ \hline
    OOD-CV~\cite{zhao2022ood}             & Real-world              & 17.25\%                                                                          & 13.75\%                                                                        & 3.28                      & 3.33                      \\ \hline
    ViewFool~\cite{dong2022viewfool}                & Synthetic               & 45.40\%                                                                          & 37.08\%                                                                        & 2.00                      & 2.10                      \\
    GMVFool~\cite{ruan2023towards}                 & Synthetic               & 61.92\%                                                                          & 52.17\%                                                                        & 2.00                      & 1.00                      \\ \rowcolor{gray!25}
    AdvDreamer (Ours)              & Synthetic               & \textbf{82.00\%}                                                                          & \textbf{81.30\%}                                                                       & \textbf{2.72}                      & \textbf{2.87}                      \\ \hline
    \end{tabular}}
\label{sample compare}
\end{table}

\section{Prompt Templates}\label{sec:c}
Fig.~\ref{fig:prompt1} illustrates the prompt template for automatic annotation of NRM training data. The prompt templates for computing GPT-Score and GPT-Acc metrics, which are employed to evaluate image captioning and VQA performance in our main experiments (Tab.~\textcolor{cvprblue}{2}), are presented in Fig.~\ref{fig:prompt2}.

\begin{figure*}[t]
  \centering
  \includegraphics[height=9.7cm]{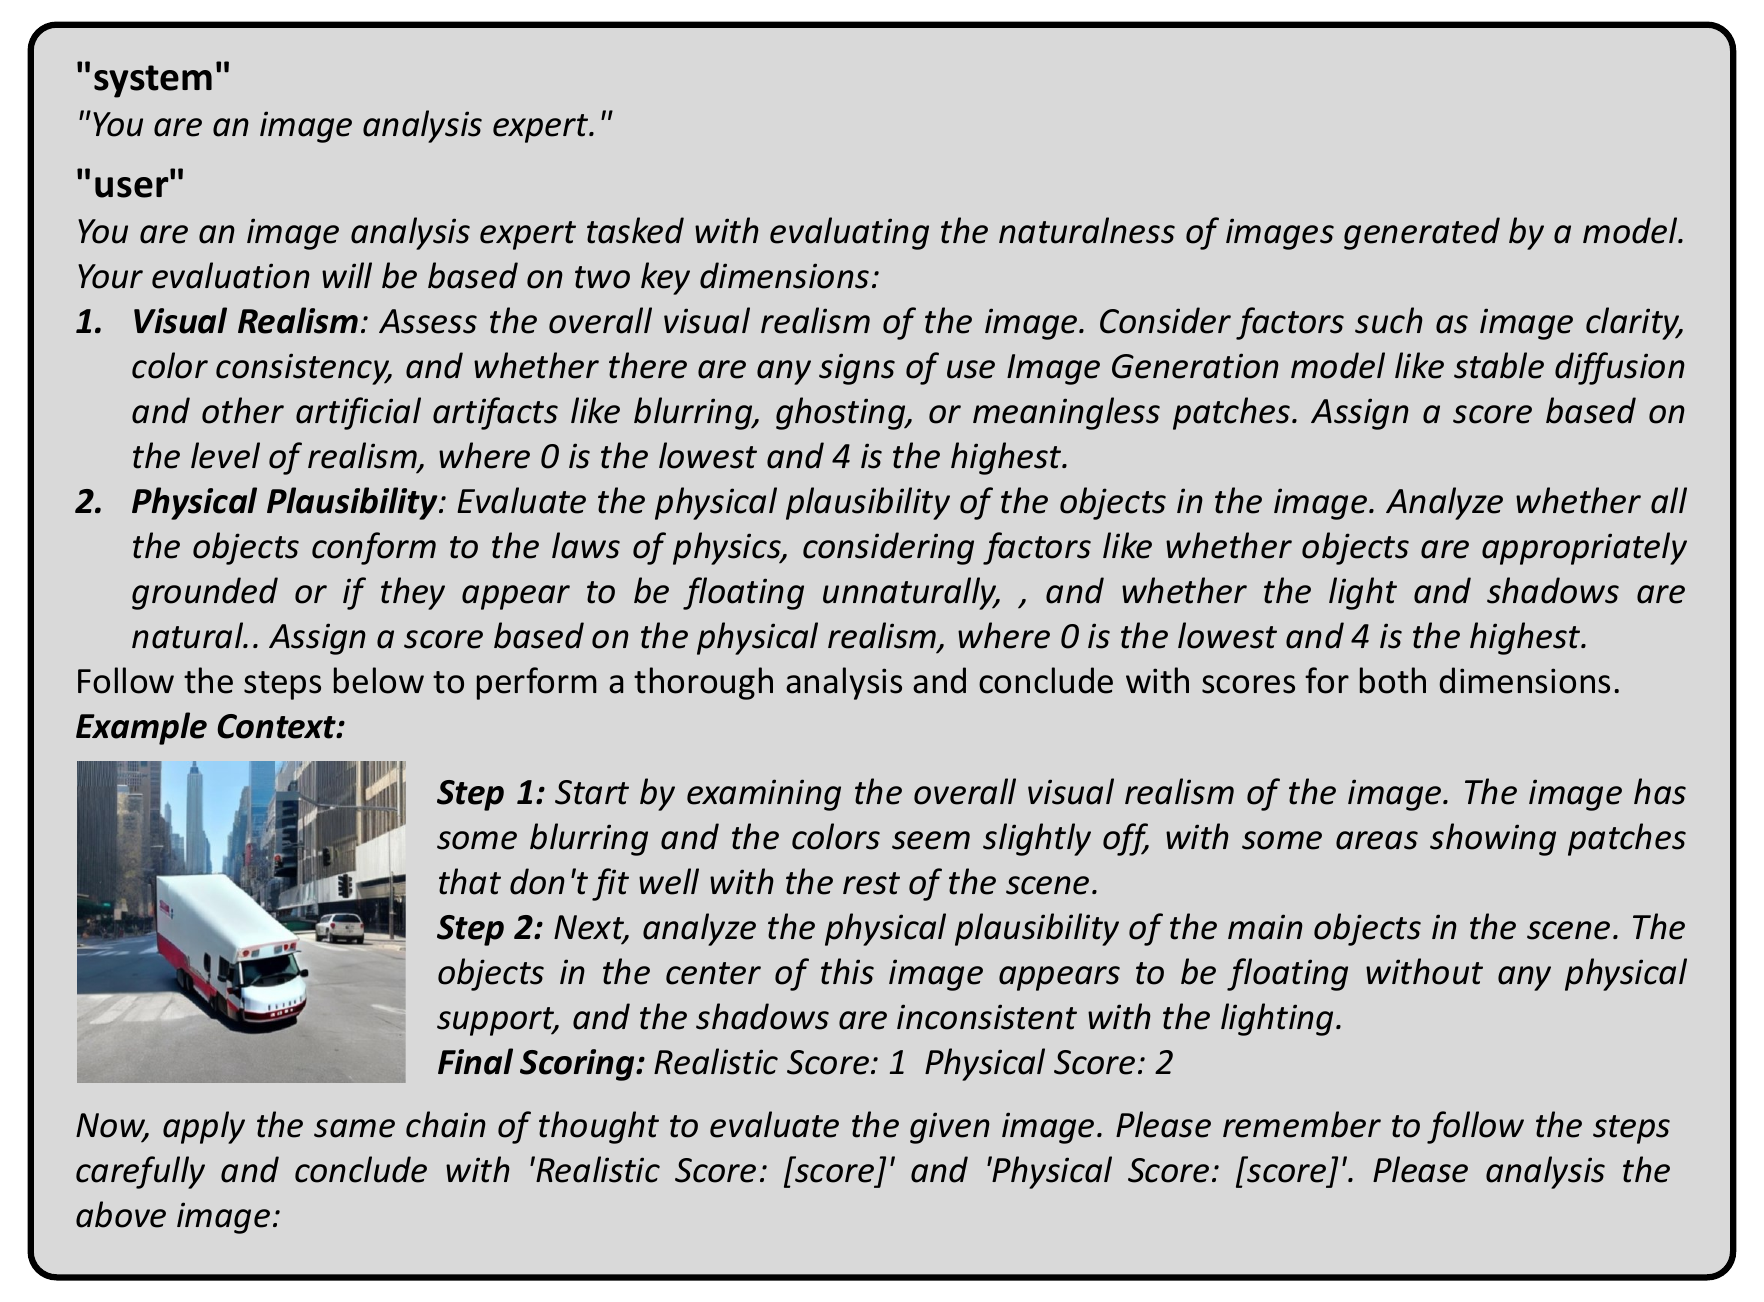}
  \caption{The prompt template for image naturalness evaluation}
  \label{fig:prompt1}
\end{figure*}
\begin{figure*}[ht]
  \centering
  \includegraphics[height=10.1cm]{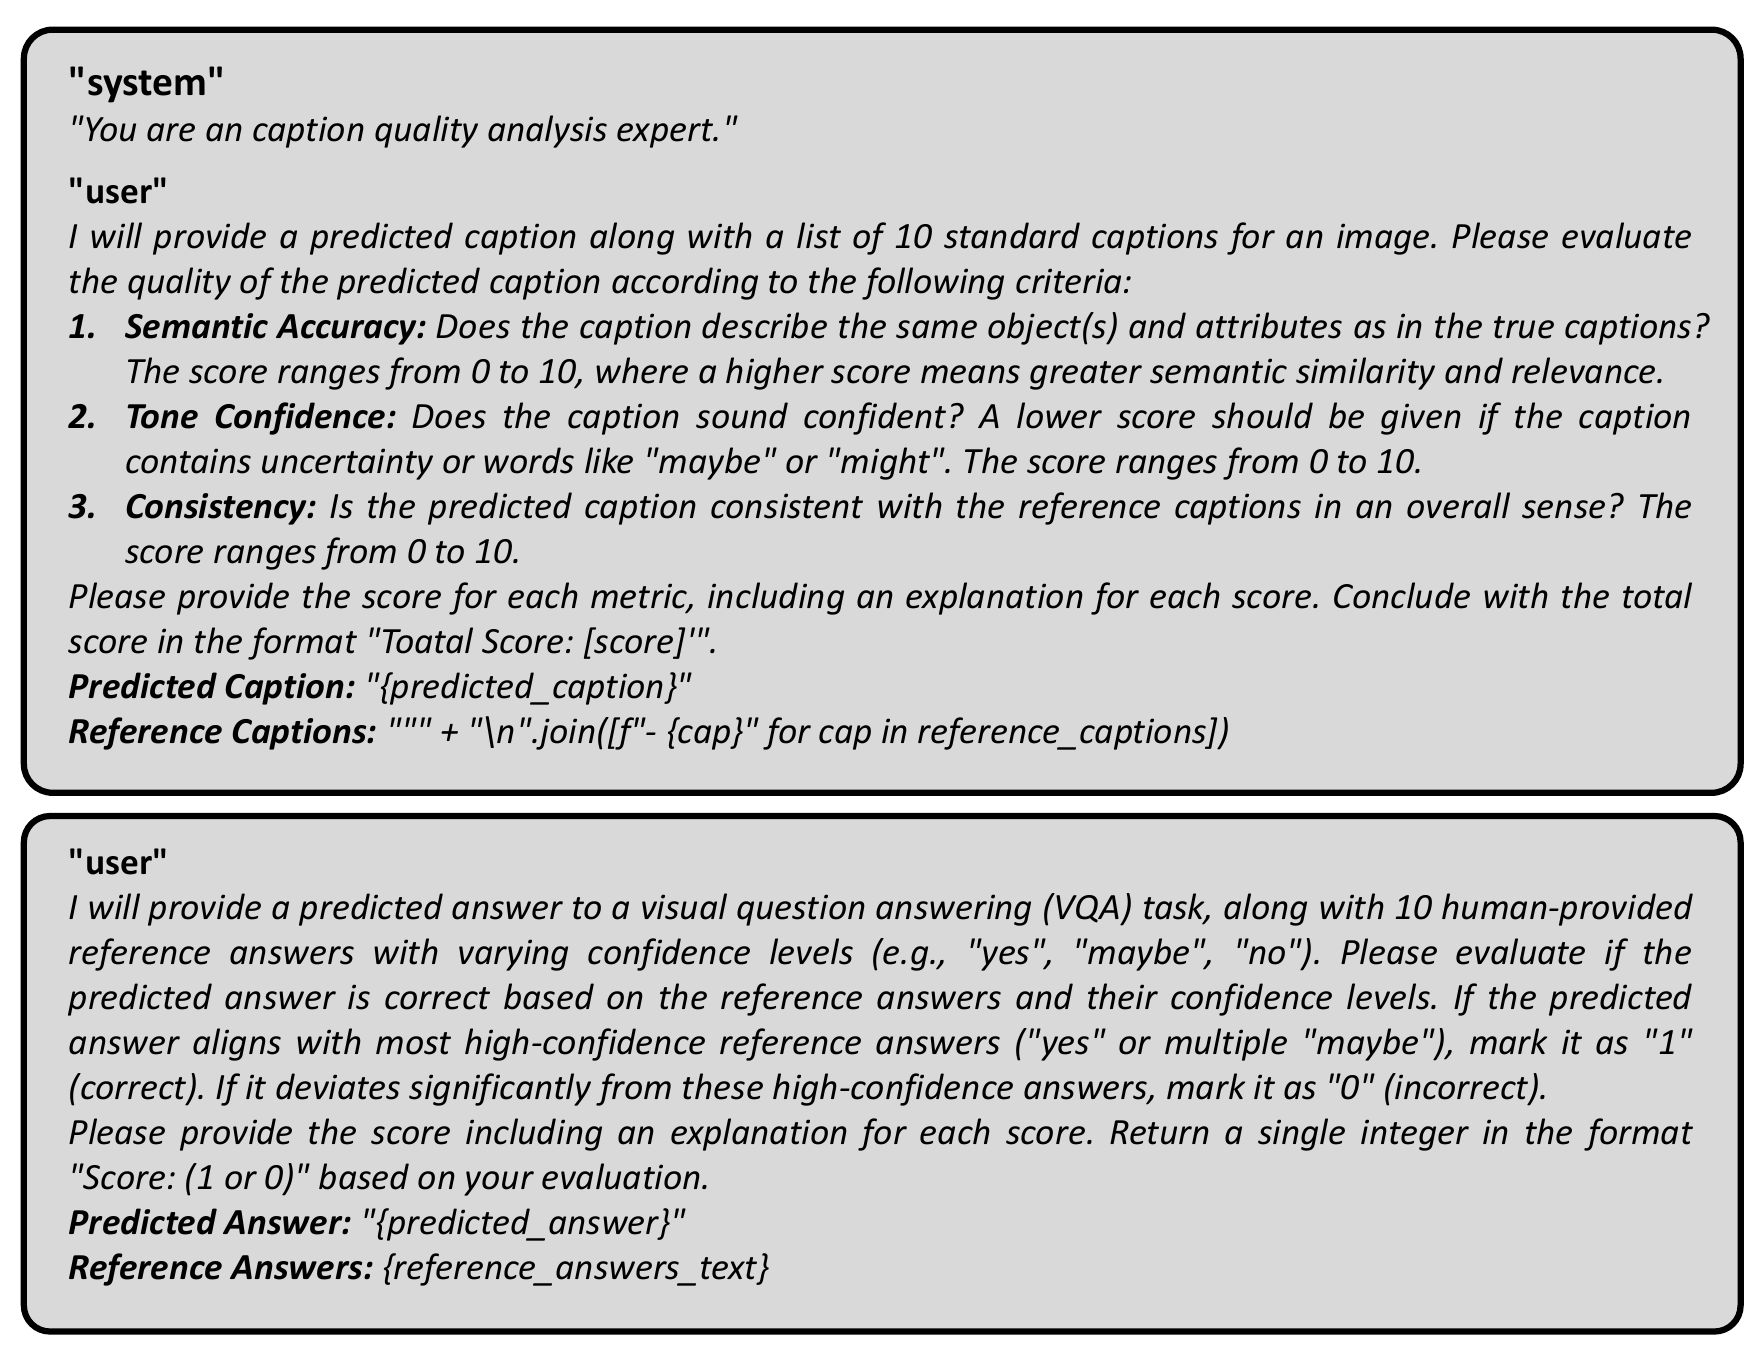}
  \caption{The prompt template for GPT-Score in image captioning tasks and for GPT-Acc in VQA tasks.}
  \label{fig:prompt2}
\end{figure*}

\section{Visualization Examples}\label{sec:d}
We provide additional visualization examples of physically captured Adv-3DT samples in Fig.~\ref{fig:vis-3}.
\begin{figure*}[t]
  \centering
  \includegraphics[height=6.9cm]{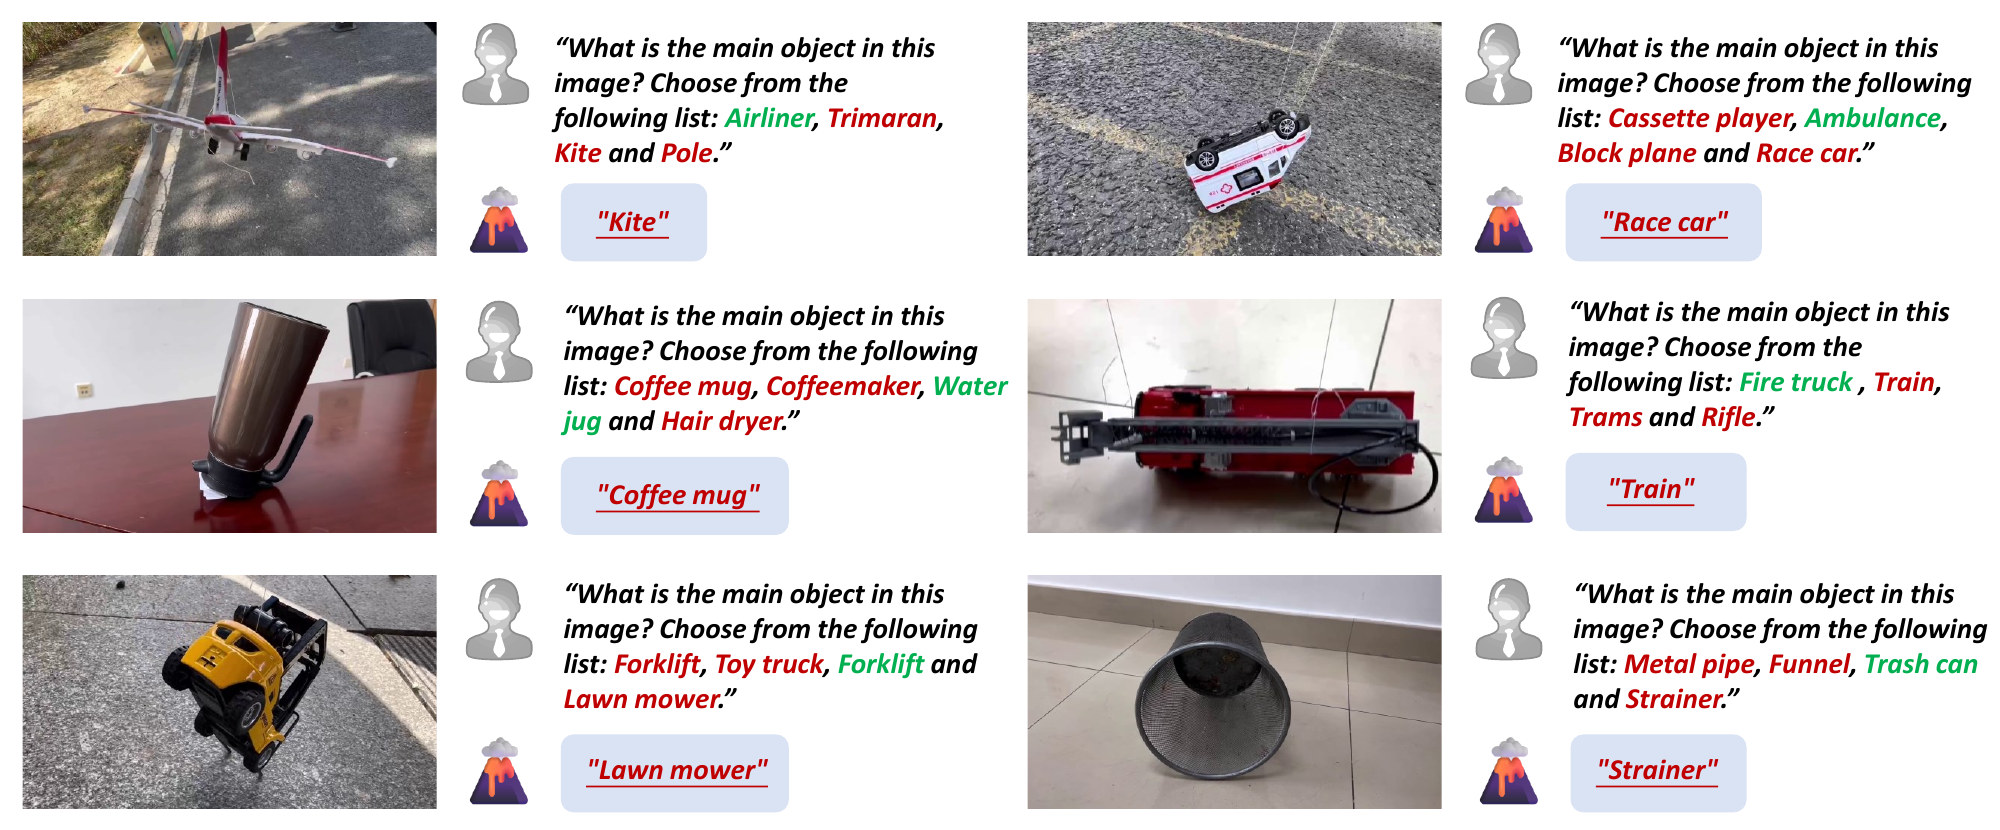}
  \caption{Additional visualization of Adv-3DT samples.}
  \label{fig:vis-3}
\end{figure*}

\section{MM3DTBench}\label{sec:e}

Tab.~\ref{bench} presents comprehensive evaluation results of representative VLMs on our MM3DTBench benchmark. To provide deeper insights into the benchmark's composition, we visualize exemplar Adv-3DT samples and their corresponding question templates and annotation format in Fig.~\ref{fig:vis-4}. The annotation framework consists of four semantic options per sample, including the ground truth label, which is carefully crafted to maintain semantic ambiguity. We also provide the spatial description of the target objects in the annotation file.

\begin{figure*}[t]
  \centering
  \includegraphics[height=7.9cm]{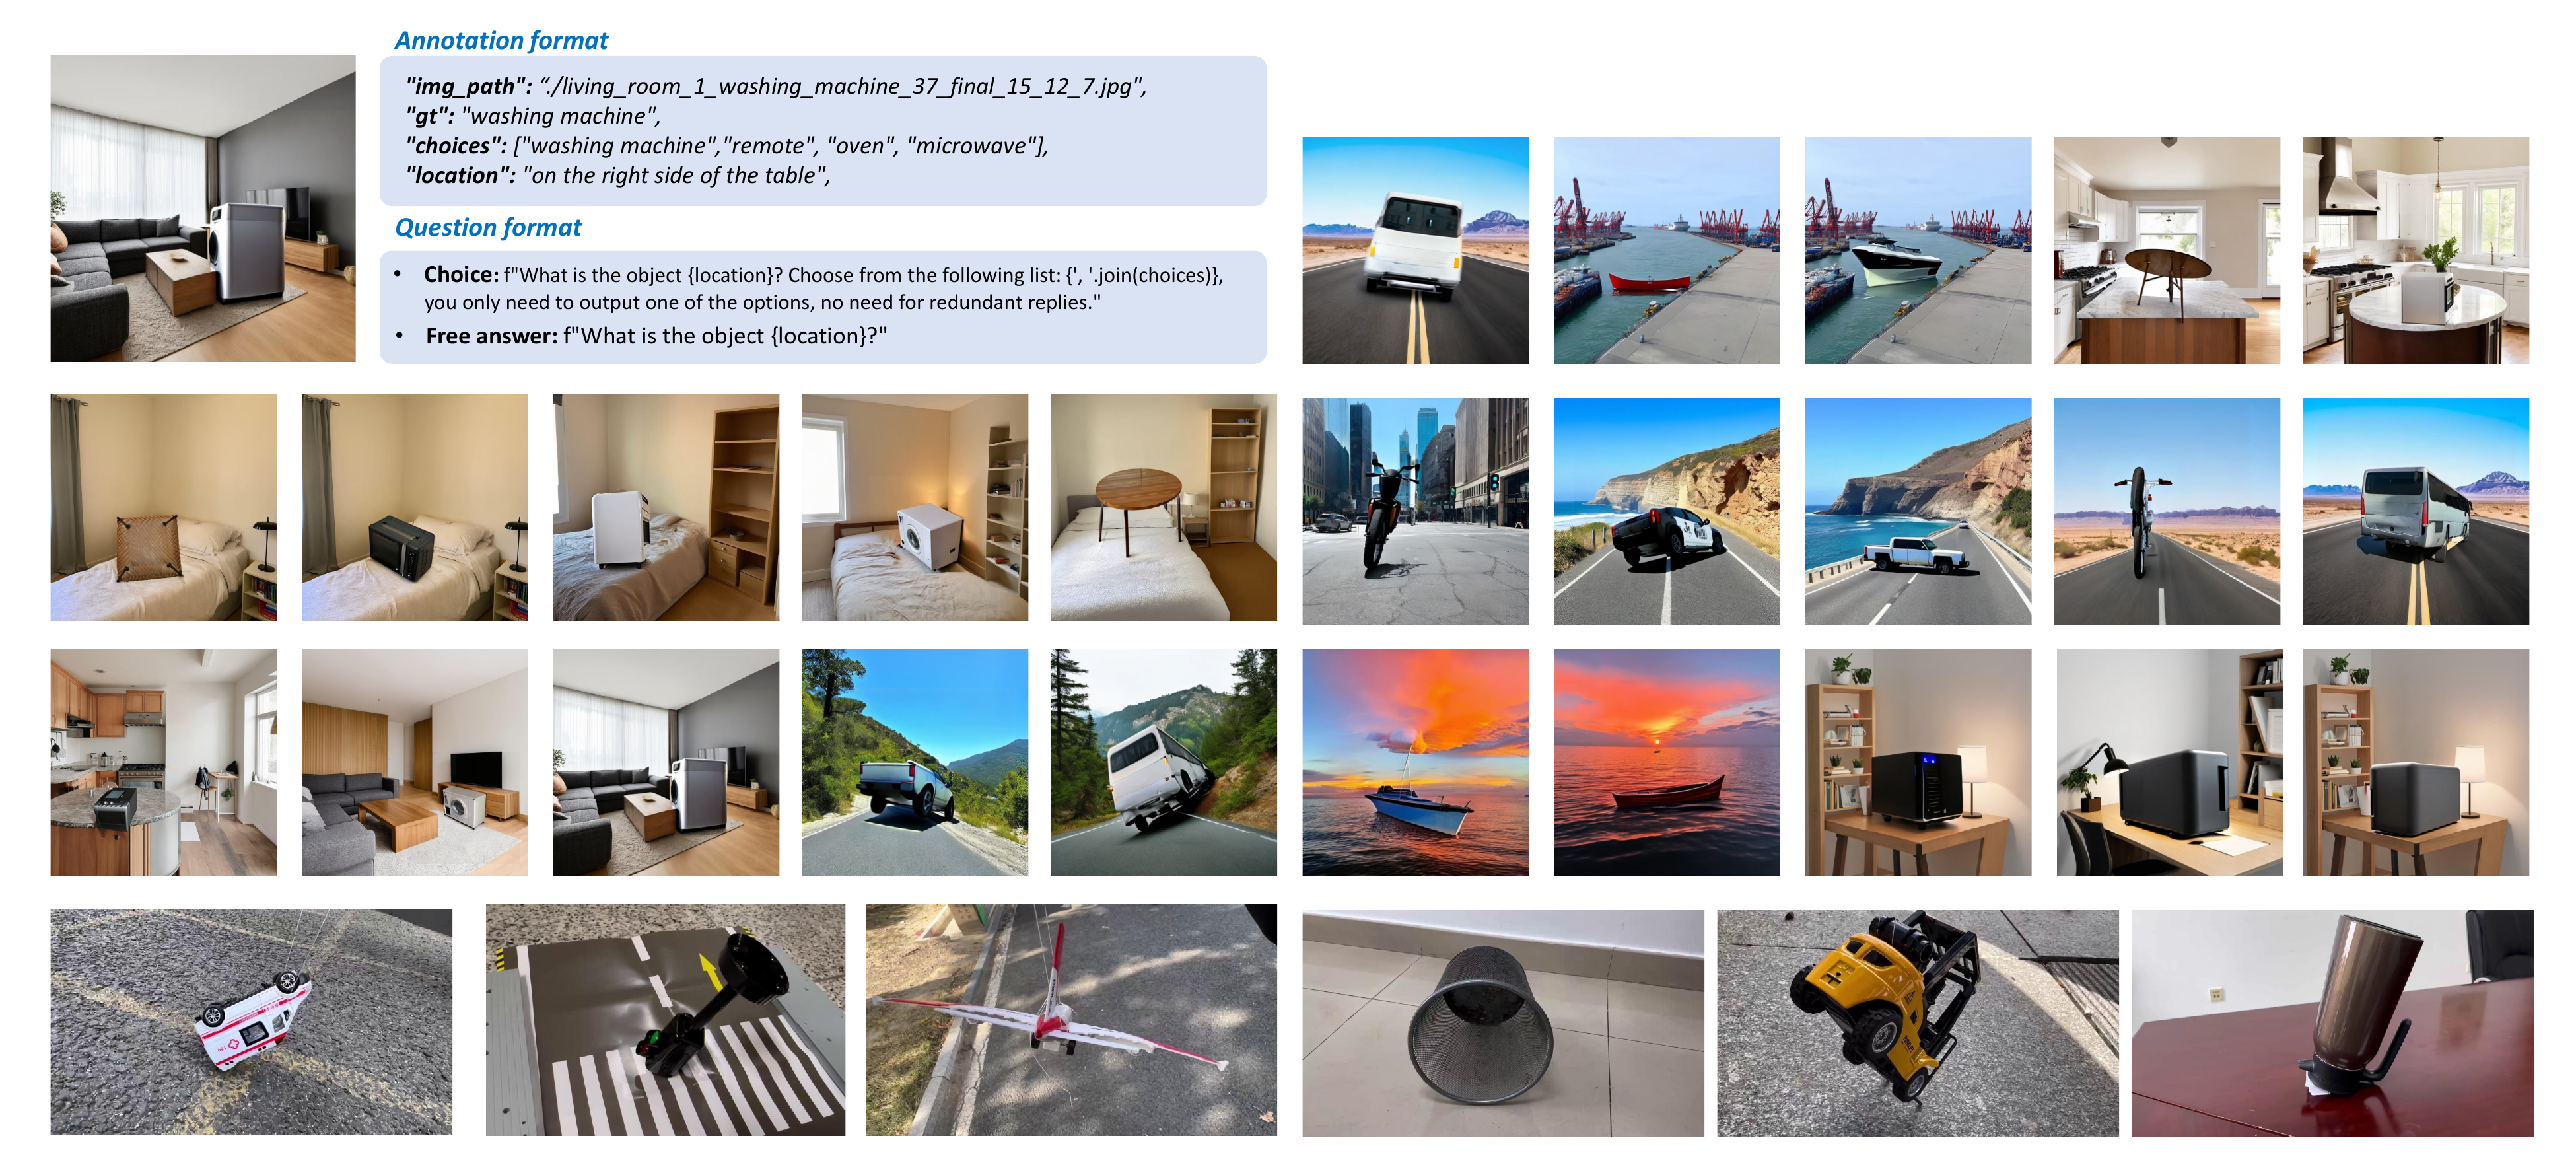}
  \caption{Anotation format, question format and some examples in MM3DTBench.}
  \label{fig:vis-4}
\end{figure*}

\clearpage

% \section{Rationale}
% \label{sec:rationale}
% % 
% Having the supplementary compiled together with the main paper means that:
% % 
% \begin{itemize}
% \item The supplementary can back-reference sections of the main paper, for example, we can refer to \cref{sec:intro};
% \item The main paper can forward reference sub-sections within the supplementary explicitly (e.g. referring to a particular experiment); 
% \item When submitted to arXiv, the supplementary will already included at the end of the paper.
% \end{itemize}
% % 
% To split the supplementary pages from the main paper, you can use \href{https://support.apple.com/en-ca/guide/preview/prvw11793/mac#:~:text=Delete%20a%20page%20from%20a,or%20choose%20Edit%20%3E%20Delete).}{Preview (on macOS)}, \href{https://www.adobe.com/acrobat/how-to/delete-pages-from-pdf.html#:~:text=Choose%20%E2%80%9CTools%E2%80%9D%20%3E%20%E2%80%9COrganize,or%20pages%20from%20the%20file.}{Adobe Acrobat} (on all OSs), as well as \href{https://superuser.com/questions/517986/is-it-possible-to-delete-some-pages-of-a-pdf-document}{command line tools}.
